# Supplementary material for: A Fourth-Order Cut-cell Multigrid Method for Solving Elliptic Equations on Arbitrary Domains
Source: arXiv:2601.02975 source file (2026-01-16)
Supplement: Supplementary file 1 [file appendix.tex]

%\section{Euler Spiral}
%\label{sec:EulerSpiral}
%Consider replacing the lower left corner of the unit box $[0,1]^2$ with a round corner.
%The round corner is a portion of the Euler spiral parameterized by
%$(x_1, x_2) = (C(2S) - C(t), s(t))$, where
%\begin{align}
%C(t) &= \int_0^t \cos \theta(\tau) ~ \rmd \tau, \\
%S(t) &= \int_0^t \sin \theta(\tau) ~ \rmd \tau, \\
%\theta(t) &= \left\{
%\begin{aligned}
%& \frac{\pi}{4} \left( \frac{t}{S} \right)^2 &&\quad 0 \le \tau \le S \\
%& \frac{\pi}{4} \left( 2 - \left( 2 - \frac{t}{S} \right)^2 \right) &&\quad S < \tau \le 2S
%\end{aligned}
%\right.,
%\end{align}
%and $t \in [0, 2S]$ is the arc length parameter.
%The other corners of the unit box are replaced similarly.

\section{Estimates on the conditioning of the sample matrices}
\label{sec:estimatesOnConditioning}

In this section we analyze the conditioning of the sample matrix
in the limit of $h \rightarrow 0$,
where $h$ is the mesh step size.
Recall that for the infinity norm we have
\begin{equation}
    \label{eq:charOfInfinityNorm}
    \lVert M \rVert_{\infty} = \max_{i} \sum_{j} \lvert M_{ij} \rvert.
\end{equation}
First we consider the one-dimensional case.
%We first present the derivation in one dimension.

Suppose $\{ x_k \}_{k=0}^n \subset \bbR$ is a collection of distinct
(hence poised) interpolation sites.
For $0 \le k \le n$, define the polynomials
\begin{equation}
    \pi_k(x) = \prod_{i=0}^{k-1} \left( x - x_i \right),
\end{equation}
with the convention $\pi_0(x) = 1$.
Suppose
\begin{equation}
    \sum_{k=0}^n a_k x^k = \sum_{k=0}^n a'_k \pi_k(x)
\end{equation}
are two identical polynomials in $\Pi_n^1$.
It is easy to see that $a_n = a'_n$ and
the mapping $\{a_k\} \rightarrow \{a'_k\}$ is invertible.
Hence $\left\{ \pi_k \right\}_{k=0}^{n}$ is also a basis of $\Pi_n^1$.
The inverse of the sample matrix can be written out explicitly
through one-dimensional divided difference:
\begin{equation}
    M^{-1}\left( \{\pi_k\}; \{x_k\} \right) =
    \begin{bmatrix}
        1 & & & \\
        \frac{-1}{x_1 - x_0} & \frac{1}{x_1 - x_0} & & \\
        \frac{1}{(x_2-x_0)(x_1-x_0)} &
        -\frac{1}{x_2-x_0}\left( \frac{1}{x_2-x_1} + \frac{1}{x_1-x_0} \right) &
        \frac{1}{(x_2-x_0)(x_2-x_1)} & \\
         & & & \ddots
    \end{bmatrix}.
    \label{eq:oneDimDividedQuot}
\end{equation}
If $y_k = c + h x_k$, we can define $\{\pi'_k\}$ to be the basis
associated with $\{y_k\}$ accordingly.
It is then clear from (\ref{eq:oneDimDividedQuot}) that
\begin{align}
    \label{eq:basisChange_2}
    M^{-1}\left(\{\pi'_k\}; \{y_k\}\right) &=
    P_2 M^{-1}\left( \{\pi_k\}; \{x_k\} \right), \\
    P_2 &= \diag\left(1, h^{-1}, h^{-2}, \cdots, h^{-n} \right).
\end{align}
Now consider the following changes of basis:
\begin{align}
    \label{eq:basisChange_1}
    M^{-1}\left( \Phi_n^1; \{y_k\} \right) =
    P_1 M^{-1}\left( \{\pi'_k\}; \{y_k\} \right), \\
    \label{eq:basisChange_3}
    M^{-1}\left( \{\pi_k\}; \{x_k\} \right) =
    P_3 M^{-1}\left( \Phi_n^1; \{x_k\} \right),
\end{align}
where $\Phi_n^1$ is defined by (\ref{eq:monomialBasis}).
As noted above, both changes retain the coefficient of the highest degree.
In other words, the last rows of $P_1$ and $P_3$ are $\mathrm{e}_{n+1}^T$.
Combining (\ref{eq:basisChange_2}) (\ref{eq:basisChange_1}) (\ref{eq:basisChange_3})
we see that the last row of $M^{-1}(\Phi_n^1; \{y_k\})$ is an $h^{-n}$ multiple
of that of $M^{-1}(\Phi_n^1; \{x_k\})$.
Since $M^{-1}(\Phi_n^1; \{x_k\})$ is independent of $h$,
it follows that from (\ref{eq:charOfInfinityNorm}) that
\begin{equation}
    \left\Vert M^{-1}\left( \Phi_n^1; \{y_k\} \right) \right\Vert_{\infty}
    \ge C_0 h^{-n}
\end{equation}
for some constant $C_0$ depending on $\{x_k\}$.
But as $h \rightarrow 0^+$, %the sample matrix
$M\left( \Phi_n^1; \{y_k\} \right)$
has a limit independent of both $h$ and $\{x_k\}$.
Therefore we have
\begin{equation}
    \kappa_{\infty}\Bigl( M\left( \Phi_n^1; \{y_k\} \right) \Bigr) \ge C_1 h^{-n}
\end{equation}
for sufficiently small $h>0$.

For multi-dimensional interpolation on triangular lattices,
we have the following extension of divided difference:
\begin{theorem}[c.f.~{\cite[Theorem 5.2.2]{Phillips03}}]
    Suppose $\calT_n^D$ is a $D$-dimensional triangular lattice of degree $n$
    whose coordinates are specified by (\ref{eq:orderingOfCoordinates}).
    For $0 \le \vert \bmalpha \vert \le n$, define
    \begin{align}
        \pi_{\bmalpha}(\bmx) &= \prod_{d=1}^D \prod_{i_d=0}^{\alpha_d-1}
        \left( x_d - p_{d, i_d}\right), \\
        \label{eq:MDDividedQuoteitn}
        \left[~\right]_{\bmalpha} &= \prod_{d=1}^D \left[ p_{d,0}, \cdots, p_{d, \alpha_d} \right],
    \end{align}
    where the right-hand-side of (\ref{eq:MDDividedQuoteitn}) is the composition
    of multiple one-dimensional divided differences.
    Then the interpolant of the function $f$ on $\calT_n^D$ is given by
    \begin{equation}
        P(\bmx) = \sum_{i=0}^{n} \sum_{\vert \bmalpha \vert = i}
        \pi_{\bmalpha}(\bmx) \left[~\right]_{\bmalpha} f.
        \label{eq:multiDimInterpolant}
    \end{equation}
\end{theorem}
\begin{proof}
    We evaluate (\ref{eq:multiDimInterpolant}) on each node of the triangular lattice.
    Suppose $\bmj \in \bbZ^D$ with $0 \le \vert \bmj \vert \le n$,
    and let $\bmx_{\bmj} = \left(p_{1, j_1}, \cdots, p_{D, j_D} \right)$.
    Observe that $\pi_{\bmalpha}(\bmx_{\bmj})$ is non-zero
    only if $\bmalpha \le \bmj$ coordinate-wise.
    Hence
    \begin{equation}
%        \begin{aligned}
        P(\bmx_{\bmj}) = \sum_{\mathbf{0} \le \bmalpha \le \bmj}
        \pi_{\bmalpha}(\bmx_{\bmj}) \left[~\right]_{\bmalpha} f.
%            & = \sum_{\alpha_1 = 0}^{j_1-1} \cdots \sum_{\alpha_D = 0}^{j_D - 1}
%            \left( (x_1 - p_{1, 0}) \cdots (x_D - p_{1, j_1-1}) \right).
%        \end{aligned}
    \end{equation}
    But the right-hand-side, upon expanding, is the Newton formula
    for interpolating $f$ on the rectangular grid of
    \begin{equation}
        \left\{ p_{1, 0}, \cdots, p_{1, j_0}\right\} \times \cdots
        \times \left\{ p_{D, 0}, \cdots, p_{D, j_D} \right\}
    \end{equation}
    in a dimension-by-dimension fashion.
    Hence $P(\bmx_\bmj) = f(\bmx_\bmj)$ for all $0 \le \vert \bmj \vert \le n$.
\end{proof}
By virtue of this theorem,
the same reasoning applies to the interpolation on triangular lattices in higher dimensions.
We conclude that
\begin{equation}
    \kappa_{\infty}\Bigl( M\left( \Phi_n^D; \{\bmc + h \bmx_k\} \right) \Bigr)
    \ge C h^{-n} \quad (h \rightarrow 0^+)
\end{equation}
for $\bmc \in \bbR^D$
and $\{\bmx_k\}$ a $D$-dimensional triangular lattice of degree $n$.
